# Supplementary material for: Algorithmic Matsubara Integration for Hubbard-like models
Source: arXiv:1808.05188 ancillary file (2018-08-15)
Supplement: Supplementary file 1 [file supplemental-information-algorithmic.pdf]

# Supplemental Information: Algorithmic Matsubara Integration for Hubbard-like models

Amir Taheridehkordi,[1] S. H. Curnoe,[1] and J. P. F. LeBlanc[1,*]

[1]Department of Physics and Physical Oceanography, Memorial University of Newfoundland, St. John's, Newfoundland & Labrador A1B 3X7, Canada

(Dated: August 15, 2018)

## ALGEBRAIC OPERATIONS

The objects required to construct the full analytic result for the multi-summation over Matsubara frequencies of bare Green's functions are the $S$, $P$ and $R_n$ arrays. Knowing these arrays we need only perform three algebraic operations '$*$', '$\times$', and '$\cdot$' to obtain the analytic result of the summation as described in the main text. In this section we aim to elucidate the definitions of these operations. We consider three arrays, $H$, $C$ and $D$ with length $\ell$ given by:

$$H = [h_1, h_2, ..., h_\ell] \tag{1}$$

$$C = \Big[[c_1^1, c_1^2, ..., c_1^{m_1}], [c_2^1, c_2^2, ..., c_2^{m_2}], ..., [c_\ell^1, c_\ell^2, ..., c_\ell^{m_\ell}]\Big] \tag{2}$$

and

$$D = \Big[[d_1^1, d_1^2, ..., d_1^{m_1}], [d_2^1, d_2^2, ..., d_2^{m_2}], ..., [d_\ell^1, d_\ell^2, ..., d_\ell^{m_\ell}]\Big] \tag{3}$$

The lengths of the $i$th element of $C$ and $D$ are equal to $m_i$.

First, we define the distribution function $f$ operator on an array by its evaluation of every element of the array, for example:

$$\begin{aligned} f(C) =& f(\Big[[c_1^1, c_1^2, ..., c_1^{m_1}], [c_2^1, c_2^2, ..., c_2^{m_2}], ..., [c_\ell^1, c_\ell^2, ..., c_\ell^{m_\ell}]\Big]) \\ =& \Big[[f(c_1^1), f(c_1^2), ..., f(c_1^{m_1})], [f(c_2^1), f(c_2^2), ..., f(c_2^{m_2})], ..., [f(c_\ell^1), f(c_\ell^2), ..., f(c_\ell^{m_\ell})]\Big]. \end{aligned} \tag{4}$$

One may write down (4) in a compact form:

$$f(C)_i^j = f(C_i^j) \tag{5}$$

The operation '$*$' is defined by

$$\begin{aligned} C * D =& \Big[[c_1^1, c_1^2, ..., c_1^{m_1}], [c_2^1, c_2^2, ..., c_2^{m_2}], ..., [c_\ell^1, c_\ell^2, ..., c_\ell^{m_\ell}]\Big] * \Big[[d_1^1, d_1^2, ..., d_1^{m_1}], [d_2^1, d_2^2, ..., d_2^{m_2}], ..., [d_\ell^1, d_\ell^2, ..., d_\ell^{m_\ell}]\Big] \\ =& \Big[[c_1^1 d_1^1, c_1^2 d_1^2, ..., c_1^{m_1} d_1^{m_1}], [c_2^1 d_2^1, c_2^2 d_2^2, ..., c_2^{m_2} d_2^{m_2}], ..., [c_\ell^1 d_\ell^1, c_\ell^2 d_\ell^2, ..., c_\ell^{m_\ell} d_\ell^{m_\ell}]\Big] \end{aligned} \tag{6}$$

or

$$(C * D)_i^j = C_i^j D_i^j \tag{7}$$

The operation '$\times$' is also introduced:

$$\begin{aligned} H \times C =& [h_1, h_2, ..., h_\ell] \times \Big[[c_1^1, c_1^2, ..., c_1^{m_1}], [c_2^1, c_2^2, ..., c_2^{m_2}], ..., [c_\ell^1, c_\ell^2, ..., c_\ell^{m_\ell}]\Big] \\ =& [h_1 c_1^1, h_1 c_1^2, ..., h_1 c_1^{m_1}, h_2 c_2^1, h_2 c_2^2, ..., h_2 c_2^{m_2}, ..., h_\ell c_\ell^1, h_\ell c_\ell^2, ..., h_\ell c_\ell^{m_\ell}] \end{aligned} \tag{8}$$

Alternatively

$$(H \times C)_i^j = H_i C_i^j \tag{9}$$

Lastly, we define '·' operation:

$$H \cdot C = [h_1, h_2, ..., h_\ell] \cdot \Big[ [c_1^1, c_1^2, ..., c_1^{m_1}], [c_2^1, c_2^2, ..., c_2^{m_2}], ..., [c_\ell^1, c_\ell^2, ..., c_\ell^{m_\ell}] \Big] \\ = h_1[c_1^1, c_1^2, ..., c_1^{m_1}] + h_2[c_2^1, c_2^2, ..., c_2^{m_2}] + ... + h_\ell[c_\ell^1, c_\ell^2, ..., c_\ell^{m_\ell}] \tag{10}$$

Equivalently

$$H \cdot C = \sum_i H_i C_i. \tag{11}$$

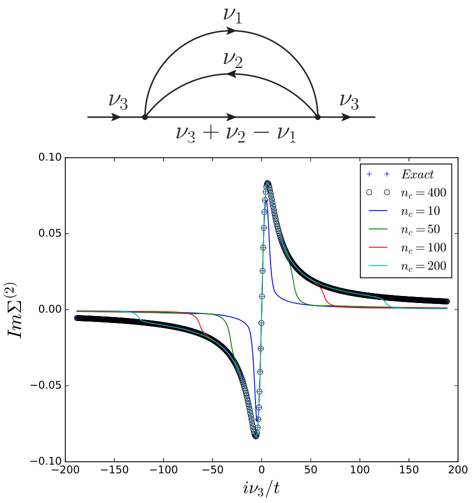


Figure S1. *Top*: Feynman diagram of $\Sigma^{(2)}$ corresponding to Eq. (12). $\nu_1$, and $\nu_2$ are independent fermionic frequencies, and $\nu_3$ is a fermionic external frequency. *Bottom*: Imaginary part of $\Sigma^{(2)}$ as a function of $\nu_3$ for crystal momentum point given in Eq. (13). The crosses show the result obtained from Eq. (16) while other lines are calculated using a finite summation with different cut-off numbers, $n_c$. As the cut-off increases the result of the finite summation converges to the exact curve calculated using AMI.

## EXAMPLES

In this section we present three examples with explicit results for the arrays $S$, $P$, and $R_n$ and demonstrate how to construct the full analytic result using AMI.

### Self Energy, $\Sigma^{(2)}$

We first evaluate an intentionally simple object, the second order Feynman diagram shown in Fig. S1. It is defined by the summation:

$$\Sigma^{(2)} = \frac{1}{\beta^2} \sum_{\nu_1,\nu_2} G(i\nu_1)G(i\nu_2)G(i\nu_3 + i\nu_2 - i\nu_1) \tag{12}$$

where $\nu_1$, $\nu_2$, and $\nu_3$ are fermionic Matsubara frequencies. We (arbitrarily) select a point in the crystal momentum at:

$$\vec{k}_1 = (0,0) \\ \vec{k}_2 = \vec{k}_3 = (\frac{\pi}{a}, \frac{\pi}{3a}). \tag{13}$$

Considering the bare Green's functions for the tight-binding Hamiltonian on a square lattice, Eq. (12) can be written as

$$\Sigma^{(2)} = \frac{1}{\beta^2} \sum_{\nu_1,\nu_2} \frac{1}{-4 + i\nu_1} \frac{1}{1 + i\nu_2} \frac{1}{-1 - i\nu_1 + i\nu_2 + i\nu_3} \tag{14}$$

where we have explicitly evaluated $\epsilon_{k_1}$, $\epsilon_{k_2}$ and $\epsilon_{k_3+k_2-k_1}$ in units of the hopping amplitude, $t$. In the array representation of Green's functions this is written as

$$\Sigma^{(2)} \rightarrow \frac{1}{\beta^2} \sum_{\nu_1,\nu_2} \Big[ [-4,1,0,0]; [1,0,1,0]; [-1,-1,1,1] \Big]. \tag{15}$$

Applying AMI we obtain the final analytic result:

$$\Sigma^{(2)} \rightarrow (S_1 * (P_1)) \times (S_2 * f(P_2)) \cdot R_2^{\Sigma} \tag{16}$$

with

$$S_1 = [1,-1] \\ S_2 = \Big[ [1,1],[1,1] \Big] \\ P_1 = [4, -1 + i\nu_2 + i\nu_3] \\ P_2 = \Big[ [-1, 5 - i\nu_3], [5 - i\nu_3, -1] \Big] \\ R_2^{\Sigma} = \Big[ [-6,0,0,1], [6,0,0,-1], [6,0,0,-1], [-6,0,0,1] \Big] \tag{17}$$

The construction of Eq. (16) is equivalent to the full analytic result in the usual representation:

$$\Sigma^{(2)} = \frac{f(4)f(-1)}{-6 + i\nu_3} + \frac{f(4)f(5 - i\nu_3)}{6 - i\nu_3} + \\ \frac{-f(-1 + i\nu_2 + i\nu_3)f(5 - i\nu_3)}{6 - i\nu_3} + \\ \frac{-f(-1 + i\nu_2 + i\nu_3)f(-1)}{-6 + i\nu_3}. \tag{18}$$

In Fig. S1 we plot $\Sigma^{(2)}$ versus external frequency, $\nu_3$ at $\beta = 10$ and $\mu = 0$ using AMI and by direct summation of Eq. (12) over internal Matsubara frequencies. As expected, by increasing the cut-off number $n_c$, the finite summation approximation results converge to the exact result computed by AMI.

### Multi-Leg Diagram, $\Lambda^{env}$

The second object we investigate is $\Lambda^{env}$ shown in Fig. S2:

$$\Lambda^{env} = \frac{1}{\beta^3} \sum_{\nu_1,\nu_2,\nu_3} G(i\nu_1)G(i\nu_2)G(i\nu_3)G(i\omega)G(i\eta)G(i\theta) \tag{19}$$

with independent frequencies $i\nu_1 \to i\nu_6$ and fully dependent labels

$$\begin{aligned} \omega &= \nu_1 + \nu_2 + \nu_3 - \nu_4 - \nu_5 - \nu_6 \\ \eta &= \nu_2 + \nu_3 - \nu_4 - \nu_6 \\ \theta &= \nu_1 + \nu_2 - \nu_4 \end{aligned} \tag{20}$$

where all the $\nu_i$ Matsubara frequencies are fermionic except for $\nu_6$ which is bosonic. We (arbitrarily) select a point in the crystal momentum at

$$\begin{aligned} \vec{k}_1 &= (0,0) \\ \vec{k}_2 = \vec{k}_3 = \vec{k}_4 = \vec{k}_5 = \vec{k}_6 &= (\frac{\pi}{a}, \frac{\pi}{3a}) \end{aligned} \tag{21}$$

Applying AMI we immediately achieve the full analytic result,

$$\Lambda^{env} \to (S_1 * f(P_1)) \times (S_2 * f(P_2)) \times (S_3 * f(P_3)) \cdot R_3^{\Lambda} \tag{22}$$

where the arrays of signs are given by

$$\begin{aligned} S_1 &= [1,1,1] \\ S_2 &= \Big[[1,1,1,1],[-1,1,1],[-1,1,1]\Big] \\ S_3 &= \Big[[1,1,1],[-1,1,-1],[-1,1,-1],[1,1,1],[-1,1,-1], \\ &[-1,1,1,-1],[-1,1,-1],[1,1,1],[1,1,1],[1,-1,1,1]\Big] \end{aligned} \tag{23}$$

and the arrays of poles are

$$\begin{aligned} P_1 &= [4, -1 - i\nu_2 - i\nu_3 + i\nu_4 + i\nu_5 + i\nu_6, 4 - i\nu_2 + i\nu_4] \\ P_2 &= \Big[[-1, -5 - i\nu_3 + i\nu_4 + i\nu_5 + i\nu_6, 4 - i\nu_3 + i\nu_4 + i\nu_6, i\nu_4], [-5 - i\nu_3 + i\nu_4 + i\nu_5 + i\nu_6, -1, 4 - i\nu_3 + i\nu_4 + i\nu_6], \\ &[i\nu_4, -1, 4 - i\nu_3 + i\nu_4 + i\nu_6]\Big] \\ P_3 &= \Big[[-1, -4 + i\nu_4 + i\nu_5 + i\nu_6, 5 + i\nu_4 + i\nu_6], [-4 + i\nu_4 + i\nu_5 + i\nu_6, -1, -5 + i\nu_5 + i\nu_6], [5 + i\nu_4 + i\nu_6, -1, 4 + i\nu_6], \\ &[-1, -5 + i\nu_5 + i\nu_6, 4 + i\nu_6], [-4 + i\nu_4 + i\nu_5 + i\nu_6, -1, -5 + i\nu_5 + i\nu_6], [-4 + i\nu_4 + i\nu_5 + i\nu_6, -1, 5 + i\nu_4 + i\nu_6, -5 + i\nu_5 + i\nu_6], \\ &[5 + i\nu_4 + i\nu_6, -1, -5 + i\nu_5 + i\nu_6], [-1, -5 + i\nu_5 + i\nu_6, 4 + i\nu_6], [-1, -5 + i\nu_5 + i\nu_6, 5 + i\nu_4 + i\nu_6], \\ &[4 + i\nu_6, 5 + i\nu_4 + i\nu_6, -1, -5 + i\nu_5 + i\nu_6]\Big] \end{aligned} \tag{24}$$

We also present the entries of $R_3^{\Lambda}$ which along with $S$ and $P$ construct the analytic result. Here we translate the array form of $R_3^{\Lambda}$ to the entries $R_3^i$ computed by AMI:

$$\begin{aligned} R_3^1 &= \frac{1}{3 - i\nu_4 - i\nu_5 - i\nu_6} \frac{1}{-6 - i\nu_4 - i\nu_6} \frac{1}{-1 - i\nu_4} \\ R_3^2 &= \frac{1}{-3 + i\nu_4 + i\nu_5 + i\nu_6} \frac{1}{-9 + i\nu_5} \frac{1}{-1 - i\nu_4} \\ R_3^3 &= \frac{1}{6 + i\nu_4 + i\nu_6} \frac{1}{9 - i\nu_5} \frac{1}{-1 - i\nu_4} \\ R_3^4 &= \frac{1}{-3 + i\nu_4 + i\nu_5 + i\nu_6} \frac{1}{-9 + i\nu_5} \frac{1}{-1 - i\nu_4} \\ R_3^5 &= \frac{1}{-3 + i\nu_4 + i\nu_5 + i\nu_6} \frac{1}{-9 + i\nu_5} \frac{1}{-4 + i\nu_5 + i\nu_6} \\ R_3^6 &= \frac{1}{1 + i\nu_4} \frac{1}{-4 + i\nu_5 + i\nu_6} \frac{1}{-9 + i\nu_5} \\ R_3^7 &= \frac{1}{6 + i\nu_4 + i\nu_6} \frac{1}{9 - i\nu_5} \frac{1}{-1 - i\nu_4} \\ R_3^8 &= \frac{1}{6 + i\nu_4 + i\nu_6} \frac{1}{9 - i\nu_5} \frac{1}{5 + i\nu_6} \end{aligned} \tag{25}$$

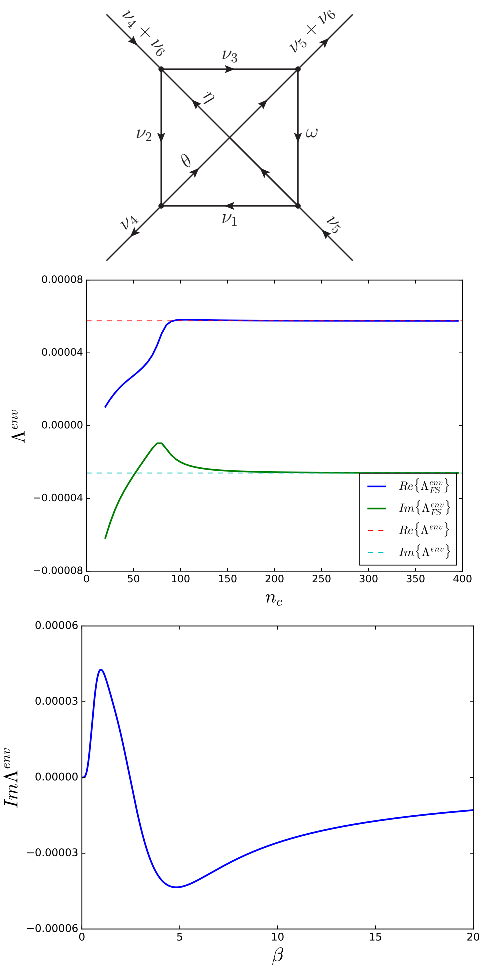


Figure S2. *Top*: Feynman diagram of $\Lambda^{env}$ given by Eq. (19). *Middle*: Imaginary and real parts of the $\Lambda^{env}$ calculated using AMI (dashed lines) and by finite summation for various cut-offs at the momenta in Eq. (21). We fix $\beta = 10$, $\mu = 0$ and the external frequencies have been set to $\nu_4 = \frac{\pi}{\beta}$, $\nu_5 = 161\frac{\pi}{\beta}$, and $\nu_6 = 0$. *Bottom*: Temperature dependence of imaginary part of $\Lambda^{env}$ calculated using AMI which approaches zero as $\beta \to \infty$.

$$R_3^9 = \frac{1}{1+i\nu_4}\frac{1}{5+i\nu_6}\frac{1}{9-i\nu_5}$$
$$R_3^{10} = \frac{1}{1+i\nu_4}\frac{1}{4-i\nu_5-i\nu_6}\frac{1}{-5-i\nu_6}$$
$$R_3^{11} = \frac{1}{1+i\nu_4}\frac{1}{-4+i\nu_5+i\nu_6}\frac{1}{-9+i\nu_5}$$
$$R_3^{12} = \frac{1}{1+i\nu_4}\frac{1}{5+i\nu_6}\frac{1}{9-i\nu_5}$$
$$R_3^{13} = \frac{1}{-3+i\nu_4+i\nu_5+i\nu_6}\frac{1}{-9+i\nu_5}\frac{1}{-1-i\nu_4}$$
$$R_3^{14} = \frac{1}{-3+i\nu_4+i\nu_5+i\nu_6}\frac{1}{-9+i\nu_5}\frac{1}{-4+i\nu_5+i\nu_6}$$

$$R_3^{15} = \frac{1}{1+i\nu_4}\frac{1}{-4+i\nu_5+i\nu_6}\frac{1}{-9+i\nu_5}$$
$$R_3^{16} = \frac{1}{-3+i\nu_4+i\nu_5+i\nu_6}\frac{1}{-9+i\nu_5}\frac{1}{-1-i\nu_4}$$
$$R_3^{17} = \frac{1}{-3+i\nu_4+i\nu_5+i\nu_6}\frac{1}{-6-i\nu_4-i\nu_6}\frac{1}{-4+i\nu_5+i\nu_6}$$
$$R_3^{18} = \frac{1}{-9+i\nu_5}\frac{1}{6+i\nu_4+i\nu_6}\frac{1}{-10-i\nu_4+i\nu_5}$$
$$R_3^{19} = \frac{1}{1+i\nu_4}\frac{1}{-4+i\nu_5+i\nu_6}\frac{1}{-10-i\nu_4+i\nu_5}$$
$$R_3^{20} = \frac{1}{-9+i\nu_5}\frac{1}{6+i\nu_4+i\nu_6}\frac{1}{-10-i\nu_4+i\nu_5}$$
$$R_3^{21} = \frac{1}{-9+i\nu_5}\frac{1}{6+i\nu_4+i\nu_6}\frac{1}{-4+i\nu_5+i\nu_6}$$
$$R_3^{22} = \frac{1}{-9+i\nu_5}\frac{1}{10+i\nu_4-i\nu_5}\frac{1}{-4+i\nu_5+i\nu_6}$$
$$R_3^{23} = \frac{1}{1+i\nu_4}\frac{1}{4-i\nu_5-i\nu_6}\frac{1}{-5-i\nu_6}$$
$$R_3^{24} = \frac{1}{1+i\nu_4}\frac{1}{-4+i\nu_5+i\nu_6}\frac{1}{-9+i\nu_5}$$
$$R_3^{25} = \frac{1}{1+i\nu_4}\frac{1}{5+i\nu_6}\frac{1}{9-i\nu_5}$$
$$R_3^{26} = \frac{1}{1+i\nu_4}\frac{1}{4-i\nu_5-i\nu_6}\frac{1}{-6-i\nu_4-i\nu_6}$$
$$R_3^{27} = \frac{1}{1+i\nu_4}\frac{1}{-4+i\nu_5+i\nu_6}\frac{1}{-10-i\nu_4+i\nu_5}$$
$$R_3^{28} = \frac{1}{1+i\nu_4}\frac{1}{6+i\nu_4+i\nu_6}\frac{1}{10+i\nu_4-i\nu_5}$$
$$R_3^{29} = \frac{1}{1+i\nu_4}\frac{1}{5+i\nu_6}\frac{1}{9-i\nu_5}$$
$$R_3^{30} = \frac{1}{1+i\nu_4}\frac{1}{6+i\nu_4+i\nu_6}\frac{1}{10+i\nu_4-i\nu_5}$$
$$R_3^{31} = \frac{1}{-5-i\nu_6}\frac{1}{6+i\nu_4+i\nu_6}\frac{1}{4-i\nu_5-i\nu_6}$$
$$R_3^{32} = \frac{1}{-9+i\nu_5}\frac{1}{10+i\nu_4-i\nu_5}\frac{1}{-4+i\nu_5+i\nu_6}$$

Fig. S2 displays the convergence of the finite summation procedure to the exact result calculated by AMI. Furthermore, the temperature dependence of imaginary part of the $\Lambda^{env}$ is presented in this figure.

We notice that the first element of the last entry of $P_2$ is purely fermionic with zero energy, and the evaluation of Fermi (bose) distribution function at this pole is formally divergent. To get around this issue one has to add a small regulator to such a pole, in this case $i\nu_4 \to i\nu_4 + \Gamma$ where $\Gamma \to 0$. In Fig. S3 we present the dependence of the $\Lambda^{env}$ to regulator $\Gamma$. As shown the result is largely independent of $\Gamma$ and the result converges to the expected value of the direct summation.

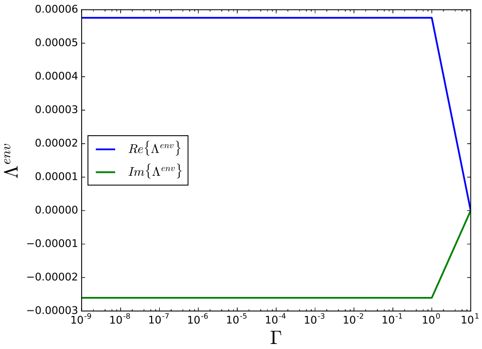


Figure S3. Imaginary and real parts of the $\Lambda^{env}$ against $\Gamma$ for a 2D square lattice ruled by tight-binding Hamiltonian, at $\beta = 10$, and $\mu = 0$ for crystal momentum point (21) computed by AMI while the external frequencies have been set to $\nu_4 = \frac{\pi}{\beta}$, $\nu_5 = 161\frac{\pi}{\beta}$, and $\nu_6 = 0$. For small enough values of $\Gamma$ both real and imaginary parts of the object do not depend on the choice of the regulator.

Table S1. Number of terms at each stage of summation assuming only simple poles, $N_{sp}$ and when treated poles with higher multiplicities, $N_{mp}$ for $J$ defined by Eq. (26) for a tight-binding Hamiltonian on a 2D square lattice at $\beta = 10$ and $\mu = 0$ at crystal momentum point $C$ given by Eq. (28). The number of terms at each stage, grows exponentially by increasing the number of summations and considering the poles' multiplicity the final analytic result includes $\sim 10^9$ terms.

| summation stage | $N_{sp}$ | $N_{mp}$ |
|---|---|---|
| 1 | 3 | 3 |
| 2 | 16 | 16 |
| 3 | 110 | 110 |
| 4 | 298 | 538 |
| 5 | 1538 | 11886 |
| 6 | 6978 | 205427 |
| 7 | 20224 | 1944668 |
| 8 | 92780 | 56109709 |
| 9 | 337982 | $\sim 10^9$ |

**9th Order Diagram, *J***

As a final example we consider a high order diagram shown in Fig. S4.[1] This diagram is chosen to be intentionally complicated, as a test of the AMI method, and has nine vertices (nine integration variables) with 17

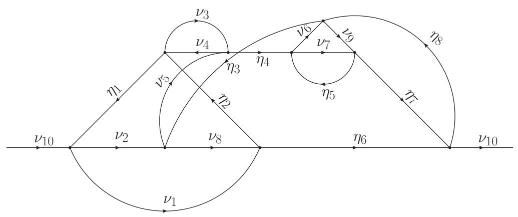


Figure S4. Feynman Diagram of $J$ defined by (26) as a ninth order diagram.

Green's functions. The summation is

$$J = \frac{1}{\beta^9} \sum_{\{\nu_i\}_{i=1}^{9}} \Big\{ G(i\nu_1)G(i\nu_2)G(i\nu_3)G(i\nu_4)G(i\nu_5)G(i\nu_6) G(i\nu_7)G(i\nu_8)G(i\nu_9)G(i\eta_1)G(i\eta_2)G(i\eta_3) G(i\eta_4)G(i\eta_5)G(i\eta_6)G(i\eta_7)G(i\eta_8) \Big\} \quad (26)$$

with

$$\begin{aligned}
\eta_1 &= \nu_1 + \nu_2 - \nu_{10} \\
\eta_2 &= \nu_1 + \nu_2 + \nu_3 - \nu_4 - \nu_{10} \\
\eta_3 &= \nu_5 + \nu_8 - \nu_2 \\
\eta_4 &= \nu_5 + \nu_3 - \nu_4 \\
\eta_5 &= \nu_6 + \nu_7 - \nu_5 - \nu_3 + \nu_4 \\
\eta_6 &= \nu_8 - \nu_2 + \nu_{10} - \nu_3 + \nu_4 \\
\eta_7 &= \nu_9 - \nu_6 + \nu_5 + \nu_3 - \nu_4 \\
\eta_8 &= \nu_5 + \nu_8 - \nu_2 + \nu_9 - \nu_6
\end{aligned} \quad (27)$$

which we evaluate at crystal momentum point $C$ given by

$$\begin{aligned}
&\vec{k}_1 = (0,0) \quad (28) \\
&\vec{k}_2 = \vec{k}_3 = \vec{k}_4 = \vec{k}_5 = \vec{k}_6 = \vec{k}_7 = \vec{k}_8 = \vec{k}_9 = (\frac{\pi}{a}, \frac{\pi}{3a}).
\end{aligned}$$

The final analytic expression for this object considering only simple poles contains 337982 terms which we do not attempt to write here. Instead we trace the number of terms at each integration stage in Table S1. We find from the third stage onwards that non-simple poles with multiplicity $M > 1$ emerge. We then construct an appropriate representation for the full analytic expression by considering the general residues for poles with multiplicity as described in the main text. When treated for multiplicity the number of terms increases dramatically from the fourth summation stage onward and by the end of the procedure the total number of terms is on the order of $10^9$. Table S1 implies that although our approach can be applied to any diagram of arbitrary complexity, in practice the presence of poles with high multiplicities (especially in the first stages of the summation) causes the computational cost to grow noticeably. In these cases, identifying where in $\{k_n\}$ space multiplicities arise will be essential to determining if evaluating a given diagram is tractable using this method.

* jleblanc@mun.ca

[1] R. Rossi, T. Ohgoe, K. Van Houcke, and F. Werner, arXiv preprint arXiv:1802.07717 (2017).
